# Supplementary material for: Climatic Extremes in Brazil: a parallel analysis of Historical Trends and Socioeconomical Impacts
Source: arXiv:2409.16309 source file (2026-06-24)
Supplement: Supplementary file 1 [file _Supplementary_Information.tex]

\documentclass[DIV=calc, paper=a4, fontsize=11pt]{scrartcl}	 % A4 paper and 11pt font size

\usepackage{geometry}
 \geometry{
 a4paper,
 total={170mm,257mm},
 left=20mm,
 top=20mm,
 bottom=30mm
 }

\usepackage[utf8]{inputenc}
\usepackage{csquotes}
\usepackage[english]{babel} % English language/hyphenation
\usepackage[protrusion=true,expansion=true]{microtype} % Better typography
\usepackage{amsmath,amsfonts,amsthm,mathrsfs} % Math packages
\usepackage[svgnames]{xcolor} % Enabling colors by their 'svgnames'
\usepackage[hang, small,labelfont=bf,up,textfont=it,up]{caption} % Custom captions under/above floats in tables or figures
\usepackage[backend=biber,style=numeric]{biblatex}
\addbibresource{sn-bibliography.bib}

\usepackage{fix-cm}	 % Custom font sizes - used for the initial letter in the document

\usepackage{graphicx}
\usepackage{scrlayer-fancyhdr} % Needed to define custom headers/footers
\pagestyle{fancy} % Enables the custom headers/footers
\usepackage{lastpage} % Used to determine the number of pages in the document (for "Page X of Total")
\usepackage{wrapfig}
\usepackage{multicol}
\usepackage{mathtools}
\usepackage{bm}
\usepackage{url}
\usepackage{braket}
\usepackage[makeroom]{cancel}
\usepackage{xcolor}
\usepackage{float}
\usepackage{subcaption}

\usepackage[normalem]{ulem}

\usepackage{glossaries}
 
\setlength{\columnwidth}{120mm}

% Headers - all currently empty
\lhead{}
\chead{}
\rhead{}

% Footers
\lfoot{}
\cfoot{}
\rfoot{\footnotesize Page \thepage\ of \pageref{LastPage}} % "Page 1 of 2"

 % No header rule
 % Thin footer rule

\usepackage{lettrine} % Package to accentuate the first letter of the text

\usepackage{titling} % Allows custom title configuration

\newcommand{\HorRule}{\color{DarkGoldenrod} \rule{\linewidth}{1pt}} % Defines the gold horizontal rule around the title

\pretitle{\vspace{-25pt} \begin{flushleft} \HorRule \fontsize{40}{40} \usefont{OT1}{phv}{b}{n} \color{DarkRed} \selectfont} % Horizontal rule before the title

%%%% TITLE
\title{\LARGE Supplementary Material \\{\large (Identification of extreme weather events and impacts of disasters in Brazil)}} 

\posttitle{\par\end{flushleft}\vskip 0.5em} % Whitespace under the title

\date{June 12th, 2024}

%----------------------------------------------------------------------------------------

\begin{document}

\maketitle 

\thispagestyle{fancy} % Enabling the custom headers/footers for the first page 

\section*{Glossary} \label{Glossary}
\begin{flushleft}
$\Delta$EE - Anomaly of Extreme Events

AP - Analysis Period: 1991-2020

EE - Extreme Events

GDP - Gross Domestic Product

INMET - Brazilian Institute of Meteorology

IPCC - Intergovernmental Panel on Climate Change

PR - Precipitation

RP - Reference Period: 1961-1990

S2iD - Brazilian Integrated System of Disasters

SM - Supplementary Material

SPEI - Standard Precipitation Evapotranspiration Index

SPEI\# - The number after SPEI indicates the time scale in months

SPI - Standard Precipitation Index

SPI\# - The number after SPI indicates the time scale in months

TN - Minimum Temperature

TN10p - Days of Extreme Minimum Temperature: TN under the temperature relative to 10\% of the percentile

TX - Maximum Temperature

TX90p - Days of Extreme Maximum Temperature: TX above the temperature relative to 90\% of the percentile

WP - Whole Period: 1961-2020

\end{flushleft}

\newpage

\section{Methods} \label{methods}

In this section we complement some information about the databases used in this work. 

\subsection*{S2iD Base} \label{s2id}

The S2iD database is the official resource when a city declares a state of calamity or catastrophe in Brazil. It is the first official dataset to be filled with information, which is later confirmed by authorities. A drawback of this database is that it is not automated and is manually filled, which can introduce errors. To address this issue, we cleaned events that were spatially and temporally close to each other, as it happened that the same event was registered twice. Additionally, in 2023, one event reported almost USD 130 billion in damages and was discarded, as this value is absurdly high compared to other EE values and the Brazilian GDP itself.

As mentioned in the main text, the S2iD database contains several entries to identify different types of disasters. In this work, we group all these types into five categories as shown in Table \ref{table_disasters}.
\begin{figure}[h!]
    \centering
    \includegraphics[width = 0.8\columnwidth]{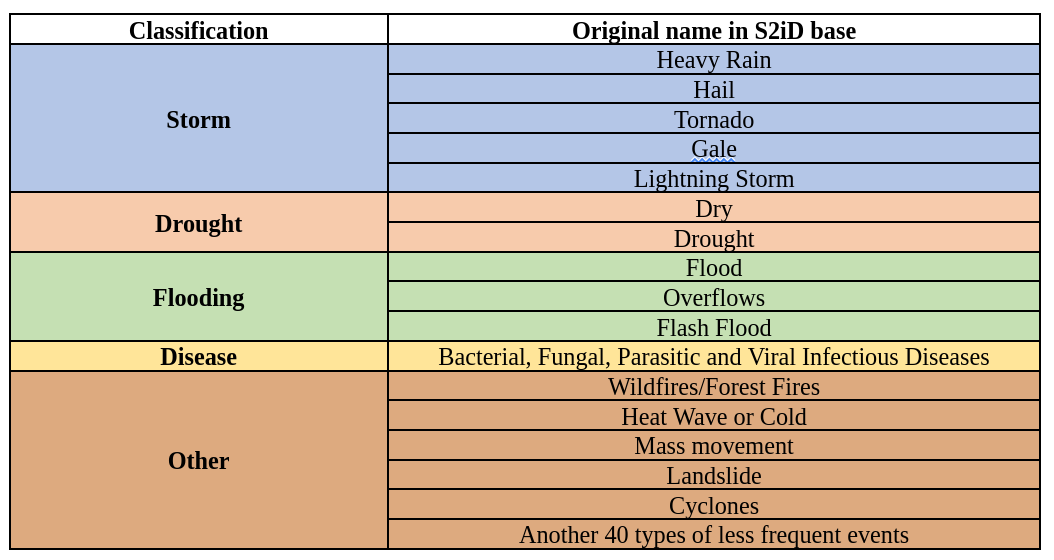}
    \caption{This table summarizes how we group different types of disasters. The left side of the table shows our classification, while the right side specifies the types of events that are registered in the S2iD. }
    \label{table_disasters}
\end{figure}

An interesting aspect of this database is that certain locations appear multiple times, as illustrated in Fig. \ref{fig_frequency_occurrences_s2id}. This may be because local authorities learn how to use the database and proceed to include every disaster that happens in their city.

 \begin{figure}
     \flushleft
     \includegraphics[width = 0.8\textwidth]{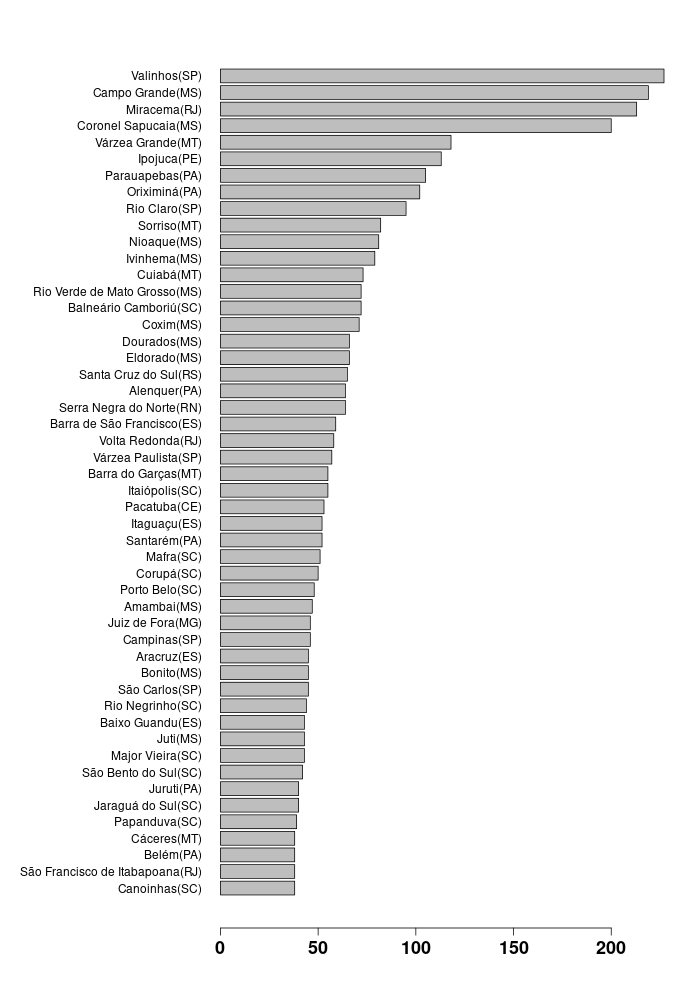}
     \caption{Sum of extreme occurrences per City and State in the time from 2013-2021 from the S2iD basis.}
     \label{fig_frequency_occurrences_s2id}
 \end{figure}

\subsection*{Exclusion of INMET meteorological stations} \label{test_cut}

As mentioned in the main text, we excluded stations with less than 30\% of data in the RP and WP and exclude individual years where a station worked for less than 30\% of the time, which resulted in approximately 287 working stations. In the next section we present the temperature extreme events (EE) indices, and show how the different exclusion criteria based on percentage of working time change EE occurrences (Fig. \ref{fig_temp_thresh_var}). Our choice of 30\% as the working time exclusion threshold is then justified as an average that retains the general trend of different threshold curves.

\section{Identification of Extreme Events}

\subsection*{Temperature Indices: TN10p and TX90p} \label{tempind}

The TN10p and TX90p are indices that reference the tails of the minimum and maximum daily temperature distributions, as described in \cite{zhang2005avoiding, WMO_2009}. They relate to the temperatures under the 10\% and over the 90\% percentiles of daily minimum (TN) and maximum (TX) temperatures, respectively. In this work, these percentiles are calculated with data only in the reference period, using a year-day window of 5 days, that define a percentile based extreme line for data in the WP. This way, the identification of EE in the analysis period takes into account what was extreme in the reference period.

\begin{figure}[h!]
    \centering
    \includegraphics[width = \textwidth]
        {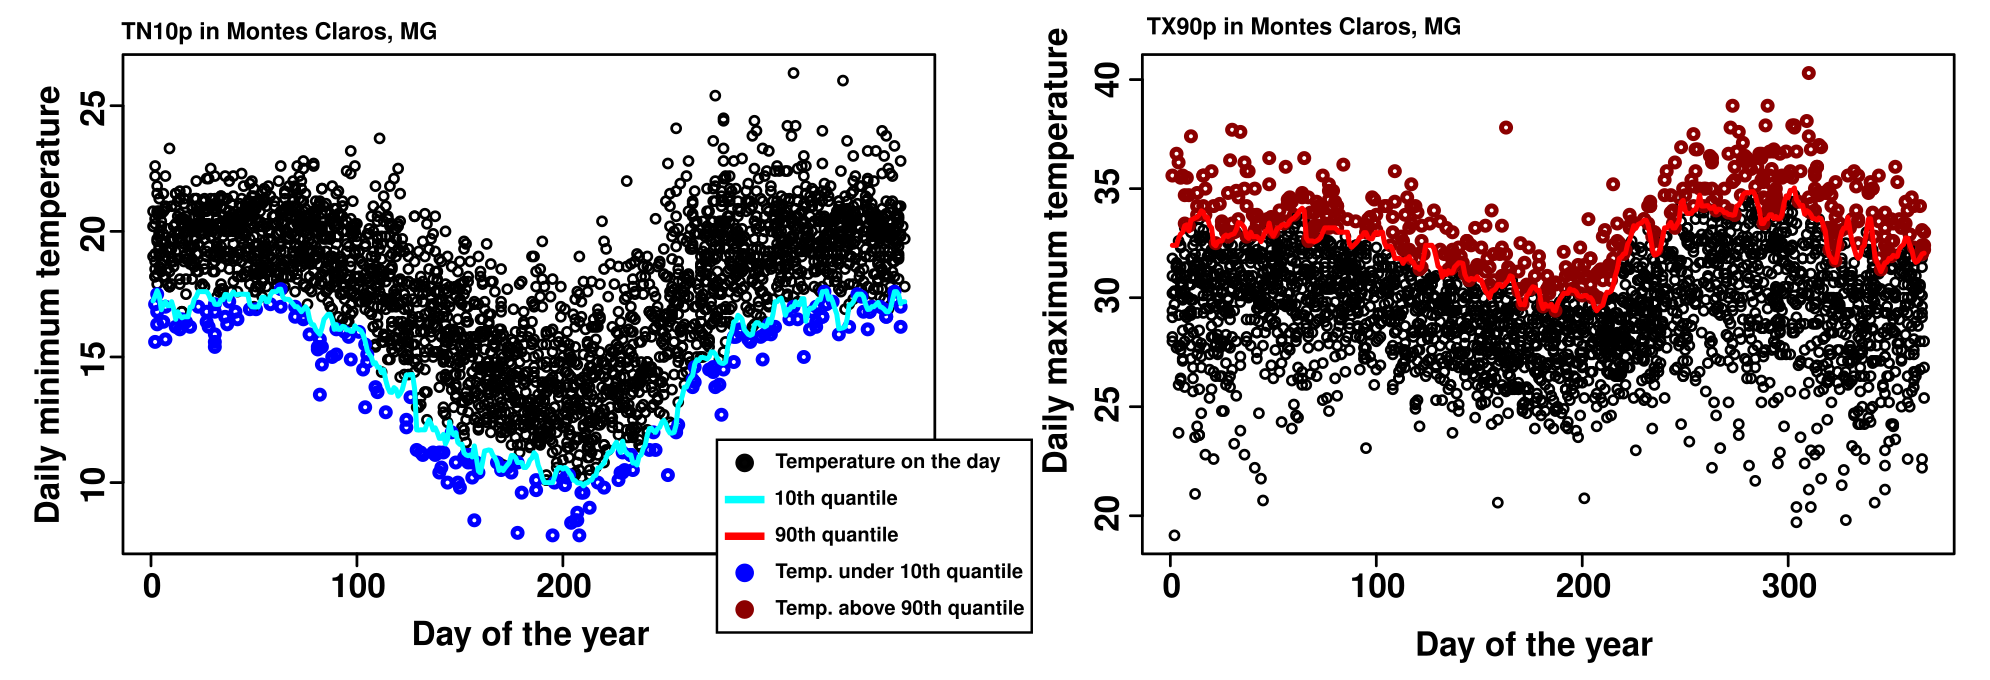}
    \caption{TN10p and TX90p EE detection threshold in a station in Montes Claros, in the state of Minas Gerais. The x axis represents days of the year (1-366), and the dots in both figures represent daily temperatures in all of the WP. The cyan and red lines in the left and right figures respectively represent the 10th and 90th data percentile, which are used as the extreme threshold. Blue points in the left figure identify minimum temperature extremes (TN10p). Red points in the right figure represent maximum temperature extremes.}
    \label{fig_temp_thresh}
\end{figure}

In Fig. \ref{fig_temp_thresh} two series of TN (left) and TX (right) are shown in the year-day representation for the RP, it organizes the daily temperature data on the day of the year (1 to 366). The figure helps to show how the indices account for seasonal effects, and how for each day of the year there is a different percentile threshold. This moving threshold is calculated using a 5-day window to increase statistics: let us suppose that day $j$ has 30 pieces of data on the TX distribution for the RP, considering the window [j-2,j+2] we increase this number to 150 pieces, which is then used to define a temperature threshold using the 90\% percentile - for instance, 36ºC for the 90\% percentile, so every TX $>$ 36ºC for day $j$ will be considered as extreme. The extreme temperature events defined on the RP are represented as blue points, under the blue line, for TN10p (on the left), and as red points, above the red line, for TX90p (on the right).

\begin{figure}[h!]
	\centering
	\includegraphics[width = \textwidth]{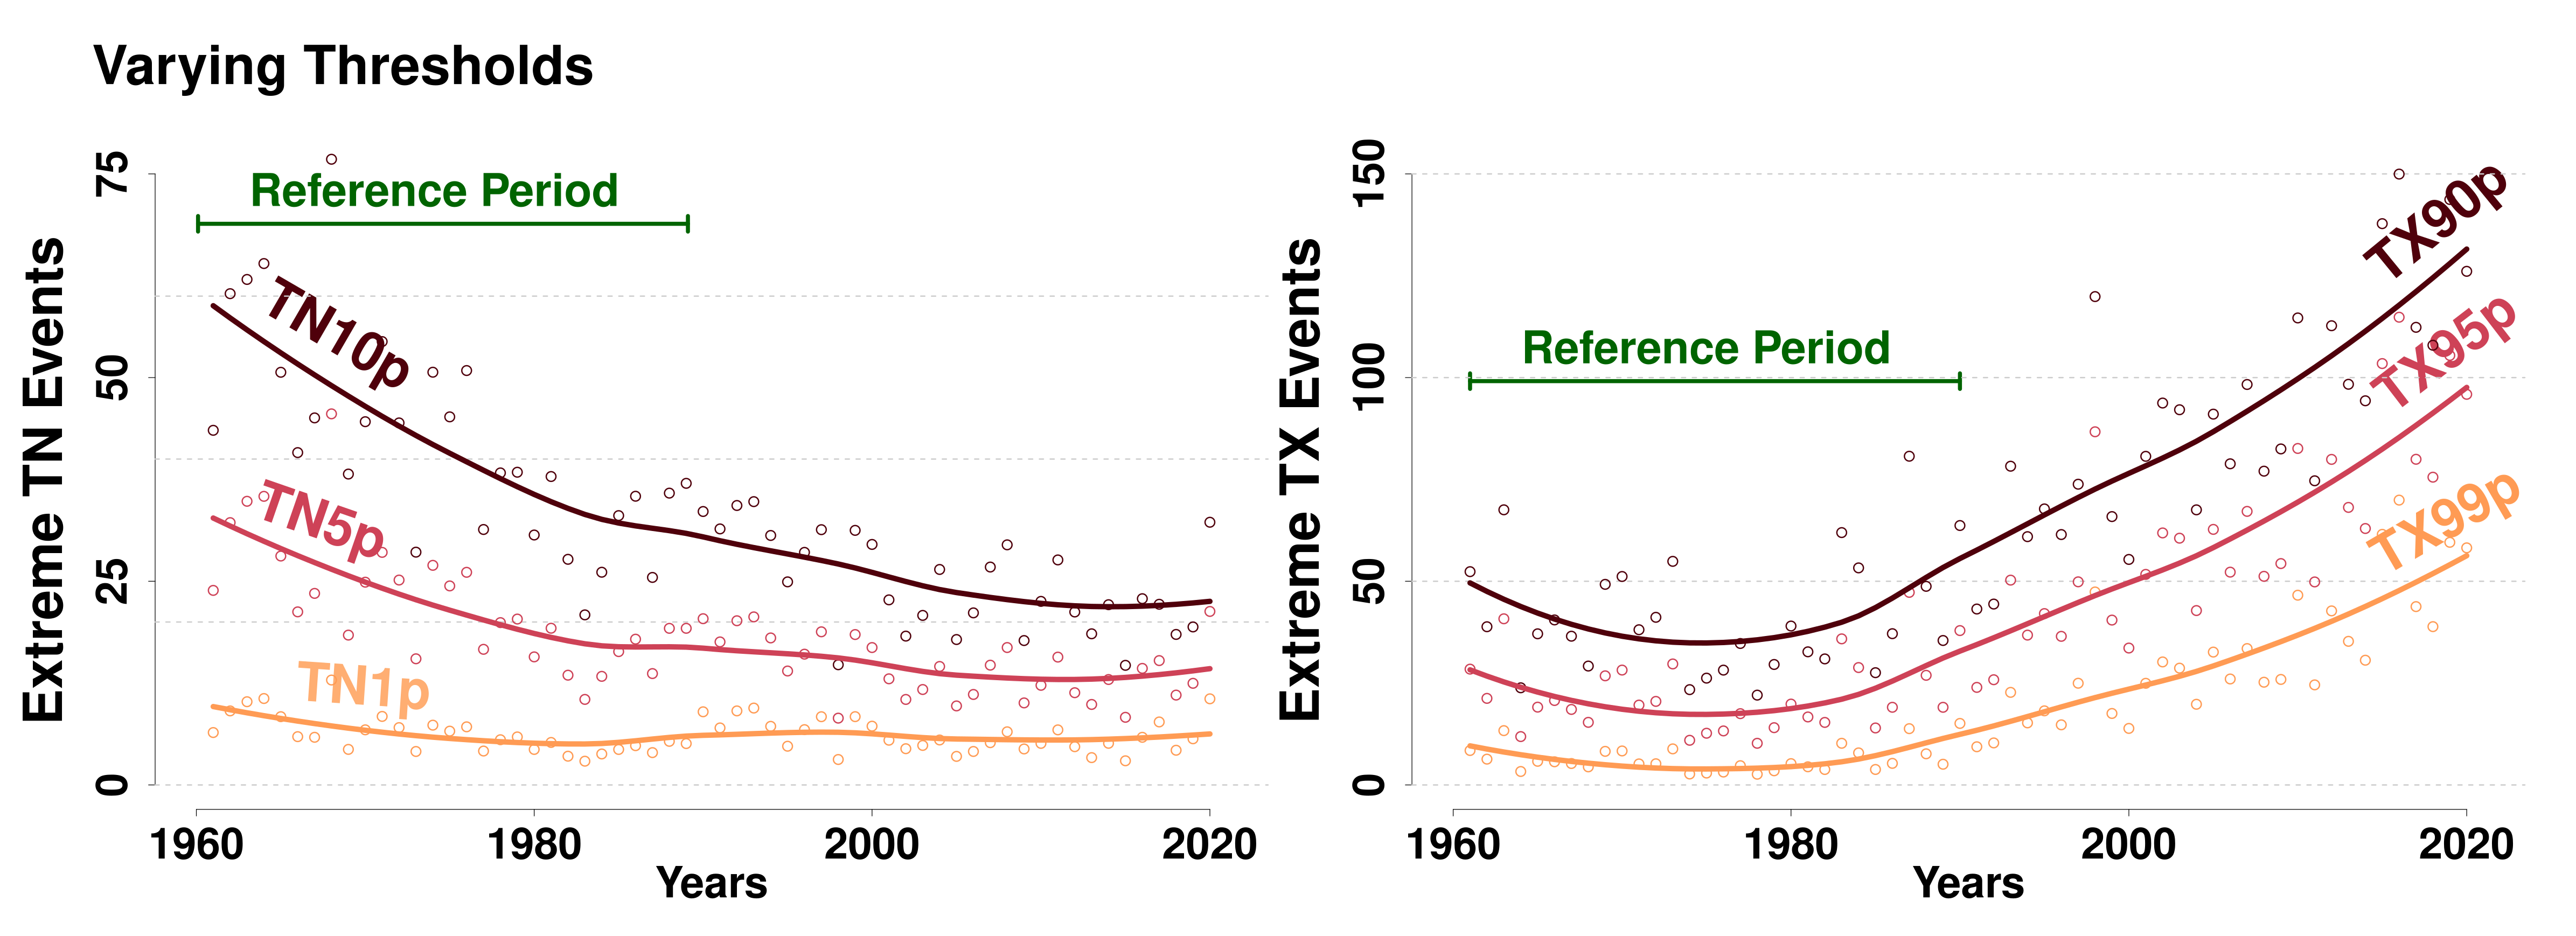}
	\caption{Both figures represent temperature series varying the extreme percentile threshold. On the left, TX is shown and the three lines represent the use of 90\%, 95\% and 99\% as thresholds. The same is done on the left using the TN and the 10\%, 5\% and 1\% thresholds.}
	\label{fig_temp_thresh_var}
\end{figure}

The Figure \ref{fig_temp_thresh_var} shows distinct time series for more rigorous extreme event thresholds (TN $<$ 1\%, 5\% and 10\% percentiles and TX $>$ 99\%, 95\% and 90\% percentiles). We see that the extreme TN events decay while extreme TX events increase independently of the percentile threshold chosen. Similarly, these results are robust for even less rigorous thresholds. As expected, the more rigorous the extreme event threshold chosen, the less events identified. Considering this, we chose the 10\% and 90\% percentile thresholds for the minimum and maximum temperatures, respectively.

\begin{figure}[H]
	\centering
	\includegraphics[width=\textwidth]{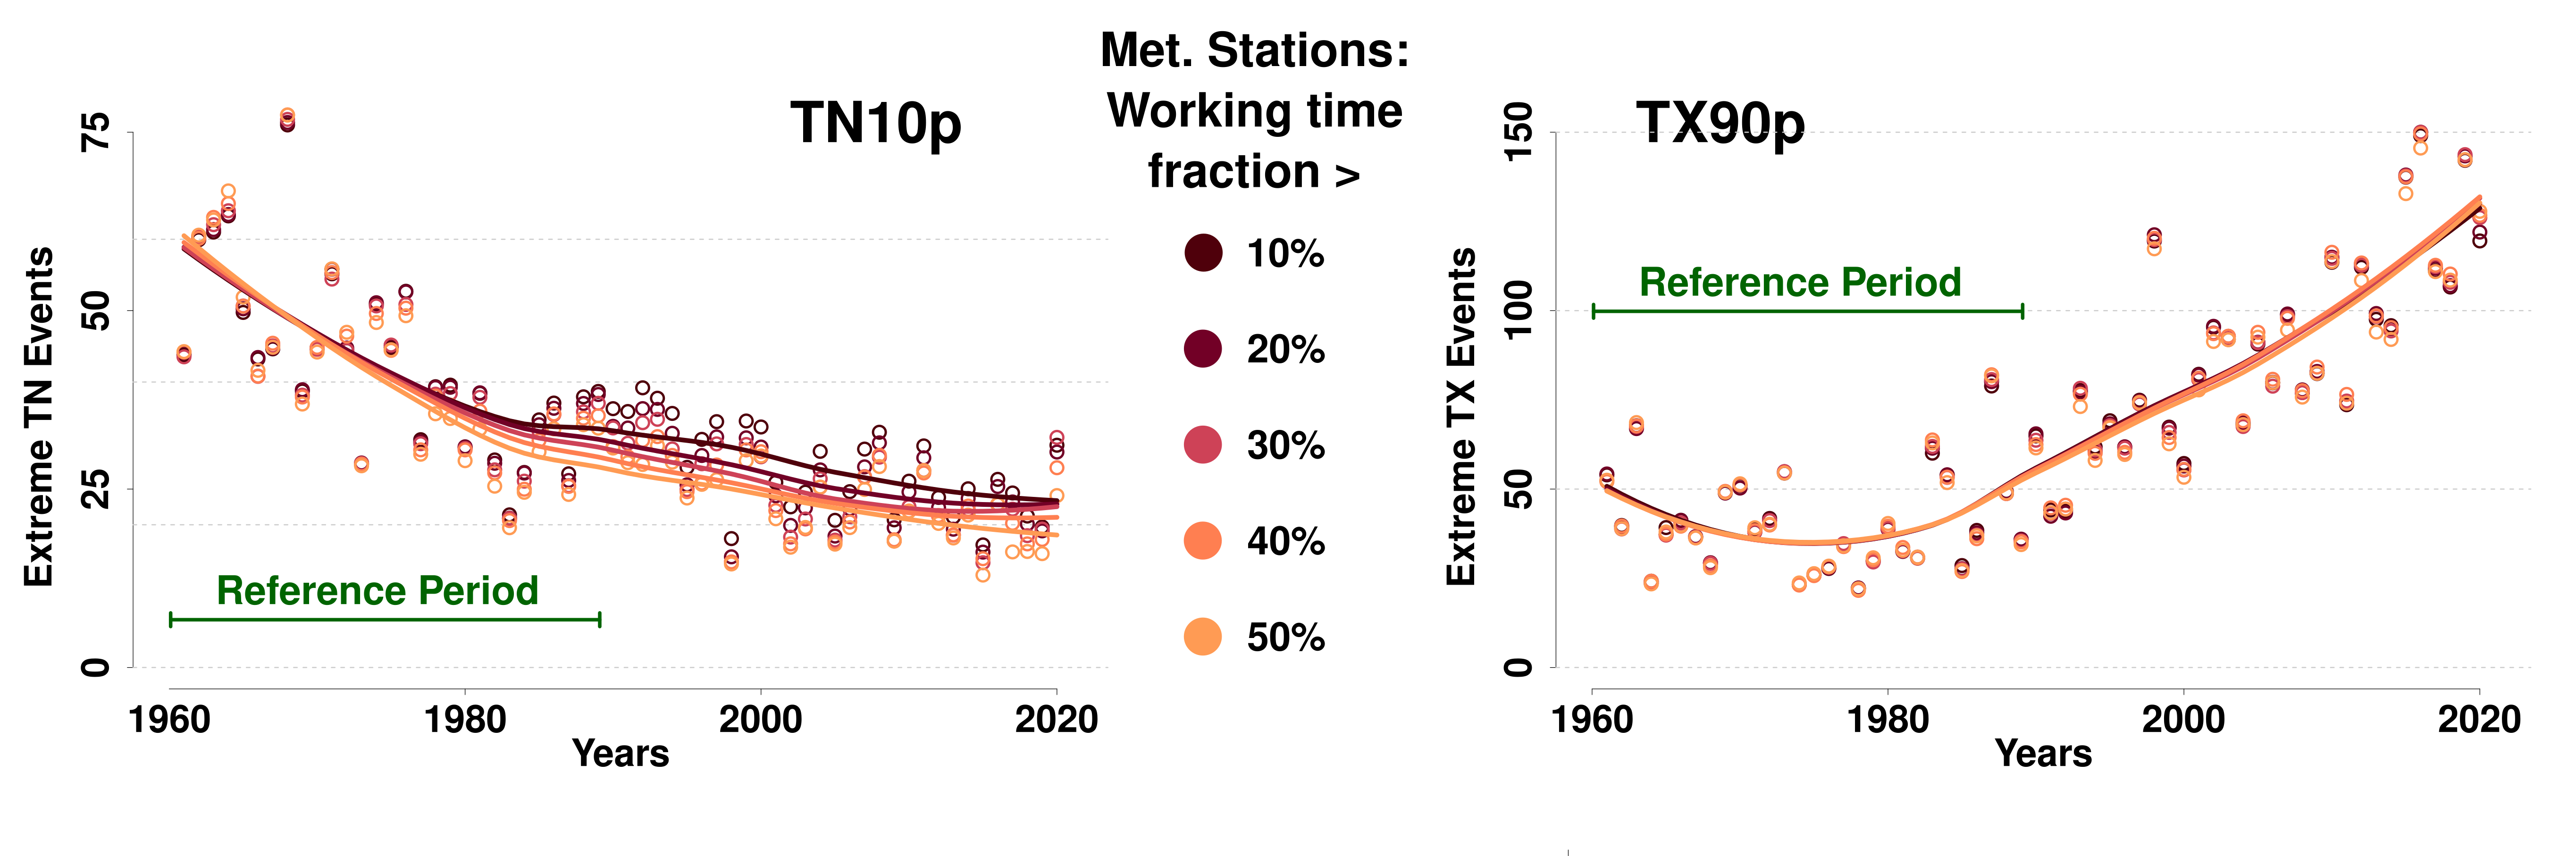}
	\caption{TX90p and TN10p EE detection varying station functioning cut. Each line and points are separated by percentage cut and identified in a particular color. The figures on the left and right represent the TN and TX behavior.}
	\label{fig_cut_vary}
\end{figure}

As mentioned in the Section \ref{test_cut}, we excluded stations which worked for less than 30\% of the WP and the RP from the whole analysis and individual years where a station worked for less than the same 30\%. To choose this fraction threshold, we tested cuts from 10-50\%, considering that different cuts could imply in changes in the EE identification. In figure \ref{fig_cut_vary}, extreme TN and TX time series are presented showing how each cut influences the data behavior. Since the general shape of the curves do not change much, in order to maintain a balance between the amount of data and the robustness of our results, the 30\% threshold was chosen.

\subsection*{Precipitation Indices: SPI and SPEI}

The precipitation indices used are the Standard Precipitation Index (SPI) and the Standard Precipitation Evapotranspiration Index (SPEI). The SPI considers only precipitation data, while the SPEI also takes temperature into account. The indices SPI3, SPEI3, SPI6, SPEI6, SPI12, and SPEI12 are calculated using the Climpact software (https://climpact-sci.org/). The numbers in the indices represent the time scales in months considered for the calculation; larger numbers correspond to longer-term droughts or wet events.
The SPI and SPEI indices are calculated based on the autocorrelation of the precipitation series, which is mapped to a normal distribution. This allows us to identify periods of autocorrelation above (blue) and below (red) a generic average, representing respectively wetter and drier periods in the region of the meteorological station. Each index defines a time window used for the autocorrelation, representing long-term (12 months, annually correlated) and short-term (3 months, seasonally correlated) dry or wet periods.

Figure \ref{fig_precipitation_indices_supp} presents an example of the plots generated by the Climpact software for Station 20 (Óbidos, PA in the North region). The y-axis indicates the magnitude of autocorrelation and the x-axis represents the years in the series. The upper graphs display SPI3 (left) and SPEI3 (right), both with the respective Sen's slope trends. The lower graphs show SPI12 (left) and SPEI12 (right), which lack sufficient data to produce the Sen's slope trends.

The trend for those series of self-correlation are tested by the Mann-Kendall test for in-homogeneous data, that is a a median over possible coefficients that do not overestimate the extremes \cite{mann1945nonparametric}, if the series pass the M-K test, the Sen's slope trend \cite{sen1968slopes} is calculated. These trends show the tendency that each station have to become drier or wetter, depending on the time scale of each index.

\begin{figure}[H]
     \centering
     \includegraphics[width=\textwidth]{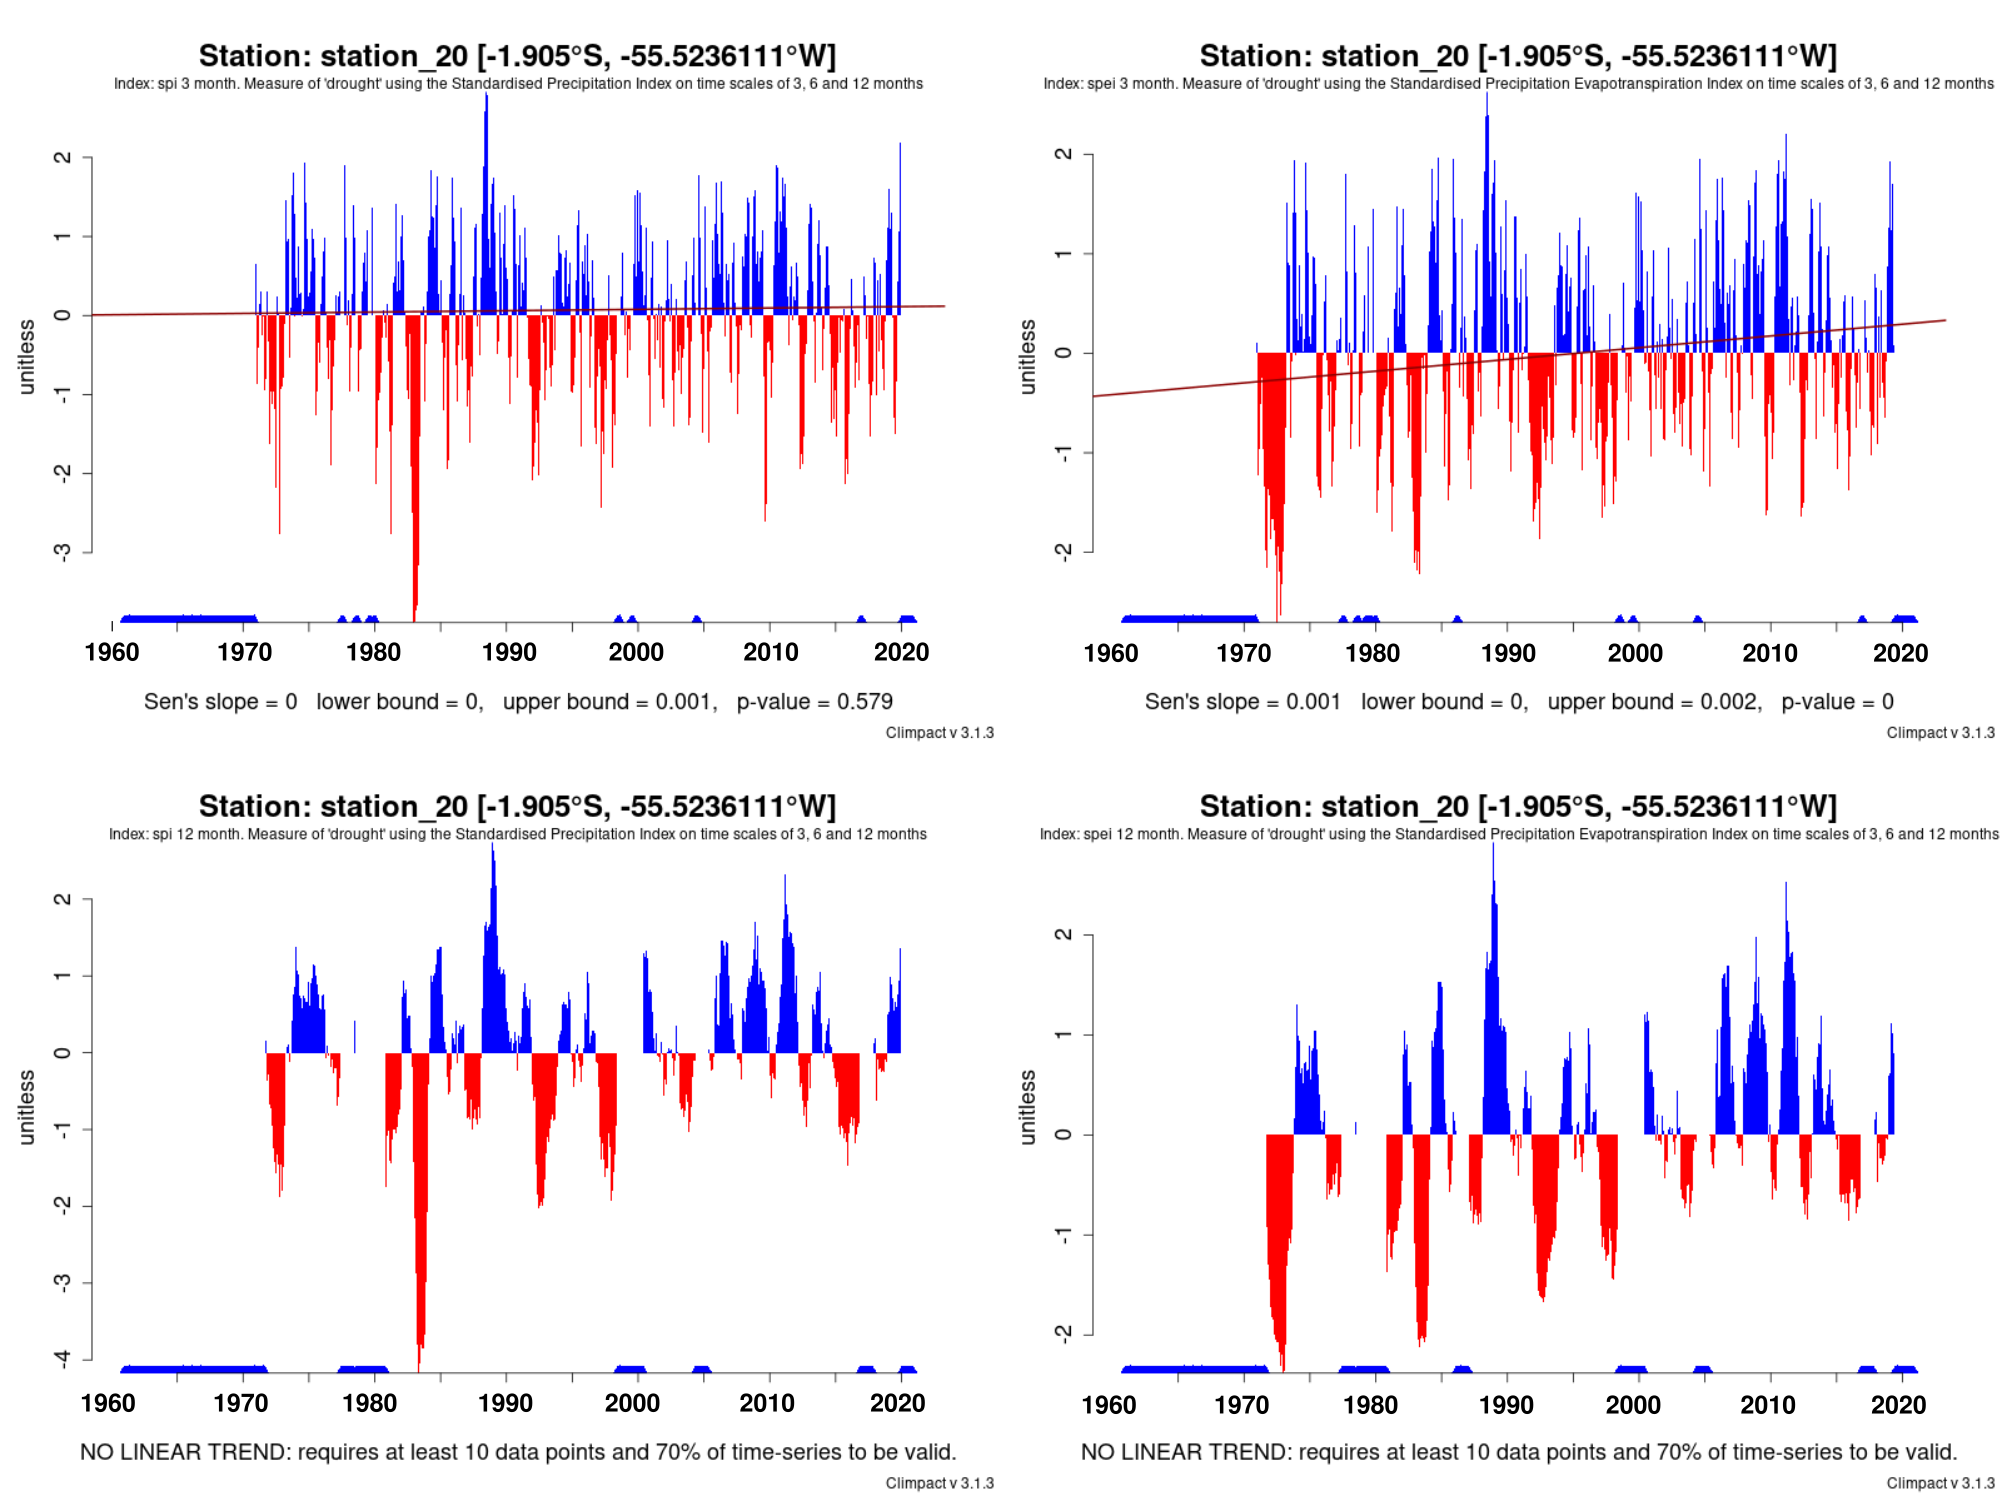}
     \caption{Examples of SPE and SPEI indexes for the metereological station 20 (Obidos, PA on the North region). The upper graphs display SPI3 (left) and SPEI3 (right), both with the respective Sen's slope trends. The lower graphs show SPI12 (left) and SPEI12 (right), which lack sufficient data to produce the Sen's slope trends.
     The y-axis represents the magnitude of autocorrelation for the precipitation series within the respective time windows (3 months for the upper panels and 12 months for the lower panels). The x-axis represents the years in the time series. Blue values indicate wet periods at this station, while red values indicate dry periods.}
    \label{fig_precipitation_indices_supp}
\end{figure}

\subsection*{Precipitation Indices: Dry days and Rain events}

The Dry Days and Rain events are indices that reference to precipitation distributions. The Dry Days extreme events are calculated using series of days without rain. In each station, the days with 0mm of precipitation are selected and days in a row are grouped. We then take the 90\% threshold of this distribution (using only data in the RP) and day series over this percentile (in the WP) are taken as extreme Dry Days events. The Rain events are the days where a station registered over 50mm of rain. These indices and the identification of extremes are both exemplified in figure \ref{fig_precip_thresh}, in an individual station in Montes Claros, Minas Gerais.

\begin{figure}[H]
    \centering
    \includegraphics[width = \textwidth]{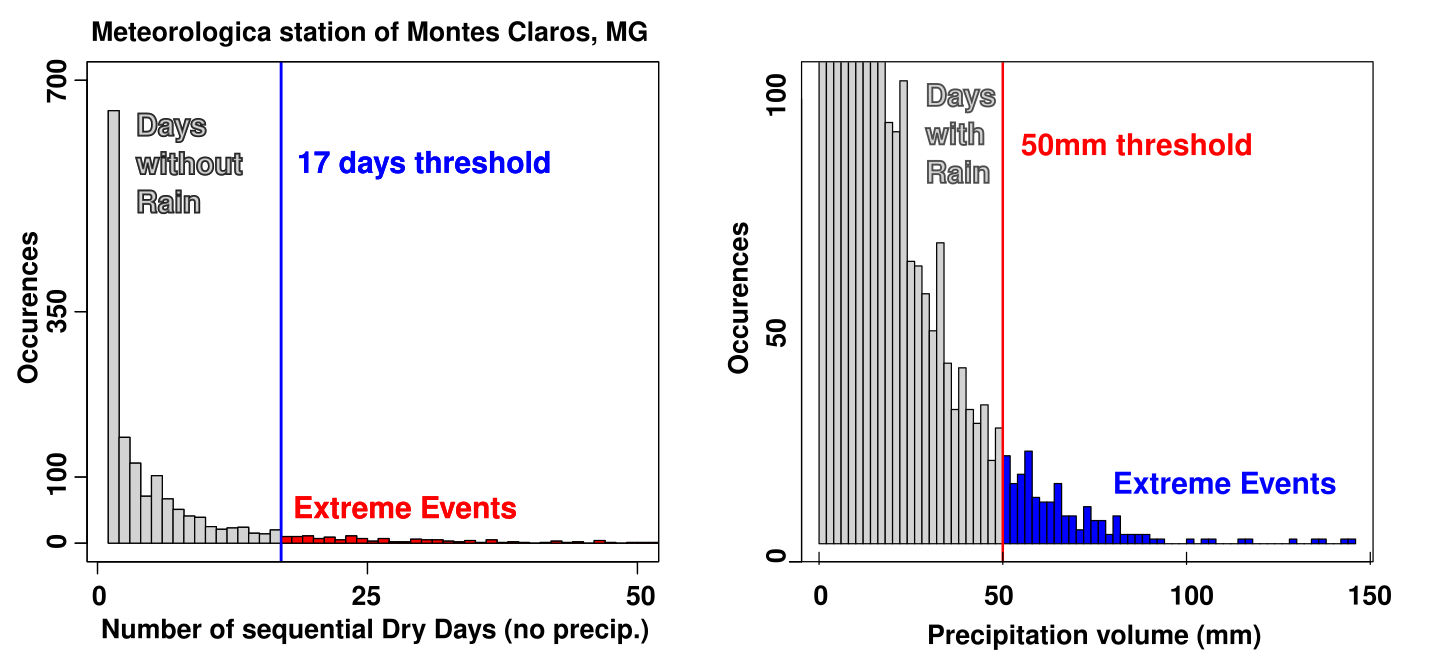}
    \caption{Dry days and Rain EE detection threshold in a station in Montes Claros, in the state of Minas Gerais. The figure on the left represent the Dry Days index, where the red line represents the number of days that mark the 90\% threshold in that station, and the red blocks represent the extreme events. On the right, the Rain index is represented, with the blue line representing 50mm of rain, used as this index's threshold, and blue blocks represent the extremes events.}
    \label{fig_precip_thresh}
\end{figure}

\subsection*{Measure of the Mean of an Extreme Event}

To calculate the mean number of EE in a given period, such as the RP or AP, we first measure the number of EE in a given station $s$ and year  $y$, ${n^{\scriptscriptstyle EE}_{\scriptscriptstyle  s,y}}$. To take into account the fact that each meteorological station does not operate the entire year,  we normalize it as follows:
\begin{equation}
N^{\scriptscriptstyle EE}_{\scriptscriptstyle  j,k} = \frac{{n^{\scriptscriptstyle EE}_{\scriptscriptstyle  s,y}}}{f_{s,y}},
\label{eq_geral}
\end{equation}
where $f_{s,y}$ is the fraction of functioning days of each station $s$ in each year $y$.

To compute the time series of EE averaged over several meteorological stations, we measure the average number of EE in a given year $y$ using the following procedure:
\begin{equation}
\overline{N^{\scriptscriptstyle EE}_{\scriptscriptstyle  y}} = \frac{\sum_s {N^{\scriptscriptstyle EE}_{\scriptscriptstyle  s,y}}}{f'_y},
\label{eq_serietemporal}
\end{equation}
where the sum is made over a range of desired meteorological stations (for example we sum up over all the stations of a Brazilian region). To take into account the fact that some stations stop working sometimes, we normalize it by $f'_y$, which is the umber of functioning stations in a given year y. Eq.(\ref{eq_serietemporal}) is used in all time series shown for TX90p, TN10p, Rain and Dry Days events.

When looking at an individual meteorological station $s$ to build the maps presented for example in Fig.2 and Fig.3 of the main text, we sum up $N^{\scriptscriptstyle EE}_{\scriptscriptstyle  j,k}$ over an interval of years $\Delta y$ and divide it by the same interval:
\begin{equation}
\overline{N^{\scriptscriptstyle EE}_{\scriptscriptstyle  s, \Delta y}} = \frac{\sum_{y \in \Delta y} N^{\scriptscriptstyle EE}_{\scriptscriptstyle s, y}}{\Delta y}.
\label{eq_serie}
\end{equation}

 In this work, Eq.(\ref{eq_serie}) is used when $\Delta y$ is the interval of time corresponding to both the AP and RP, defining the quantities used in the Eq.1 of the main text:
\begin{eqnarray}
\overline{N^{\scriptscriptstyle EE}_{\scriptscriptstyle s, RP}} = \frac{\sum_{y ~\in~ {RP}} \overline{N^{\scriptscriptstyle EE}_{\scriptscriptstyle j, k}}}{{RP}}, \\
\overline{N^{\scriptscriptstyle EE}_{\scriptscriptstyle s, AP}} = \frac{\sum_{y ~\in ~{AP}} \overline{N^{\scriptscriptstyle EE}_{\scriptscriptstyle j, k}}}{{AP}},
\label{eq_serie_RP_AP}
\end{eqnarray}
${y \in {RP}}$ (${y \in {AP}}$) indicates that the sum is over the years when station $s$ was functioning during the reference period, RP (analysis period, AP).

\section{Some results}

In this section we show some measures to complement the data shown in the main text and some figures to test the robustness of our results. 

\subsection*{Data on Temperature}

Figure \ref{fig_month_anomaly} shows the monthly temperature anomaly for all the working stations in Brazil, with each line representing an average over 5 years. The minimum temperature anomaly appears on the left and the maximum on the right, color coded from red (year 1960) to purple (year 2020). It is interesting to notice how the difference in temperature anomaly is much more pronounced in winter months (June-August), with an increase of around 4ºC for the TN anomaly and 3ºC for TX anomaly in the last sixty years, than the summer months (December-February) that have much smaller increases of around 1ºC for both temperature series on the last sixty years.

\begin{figure}[h!]
    \centering
    \includegraphics[width = \textwidth]{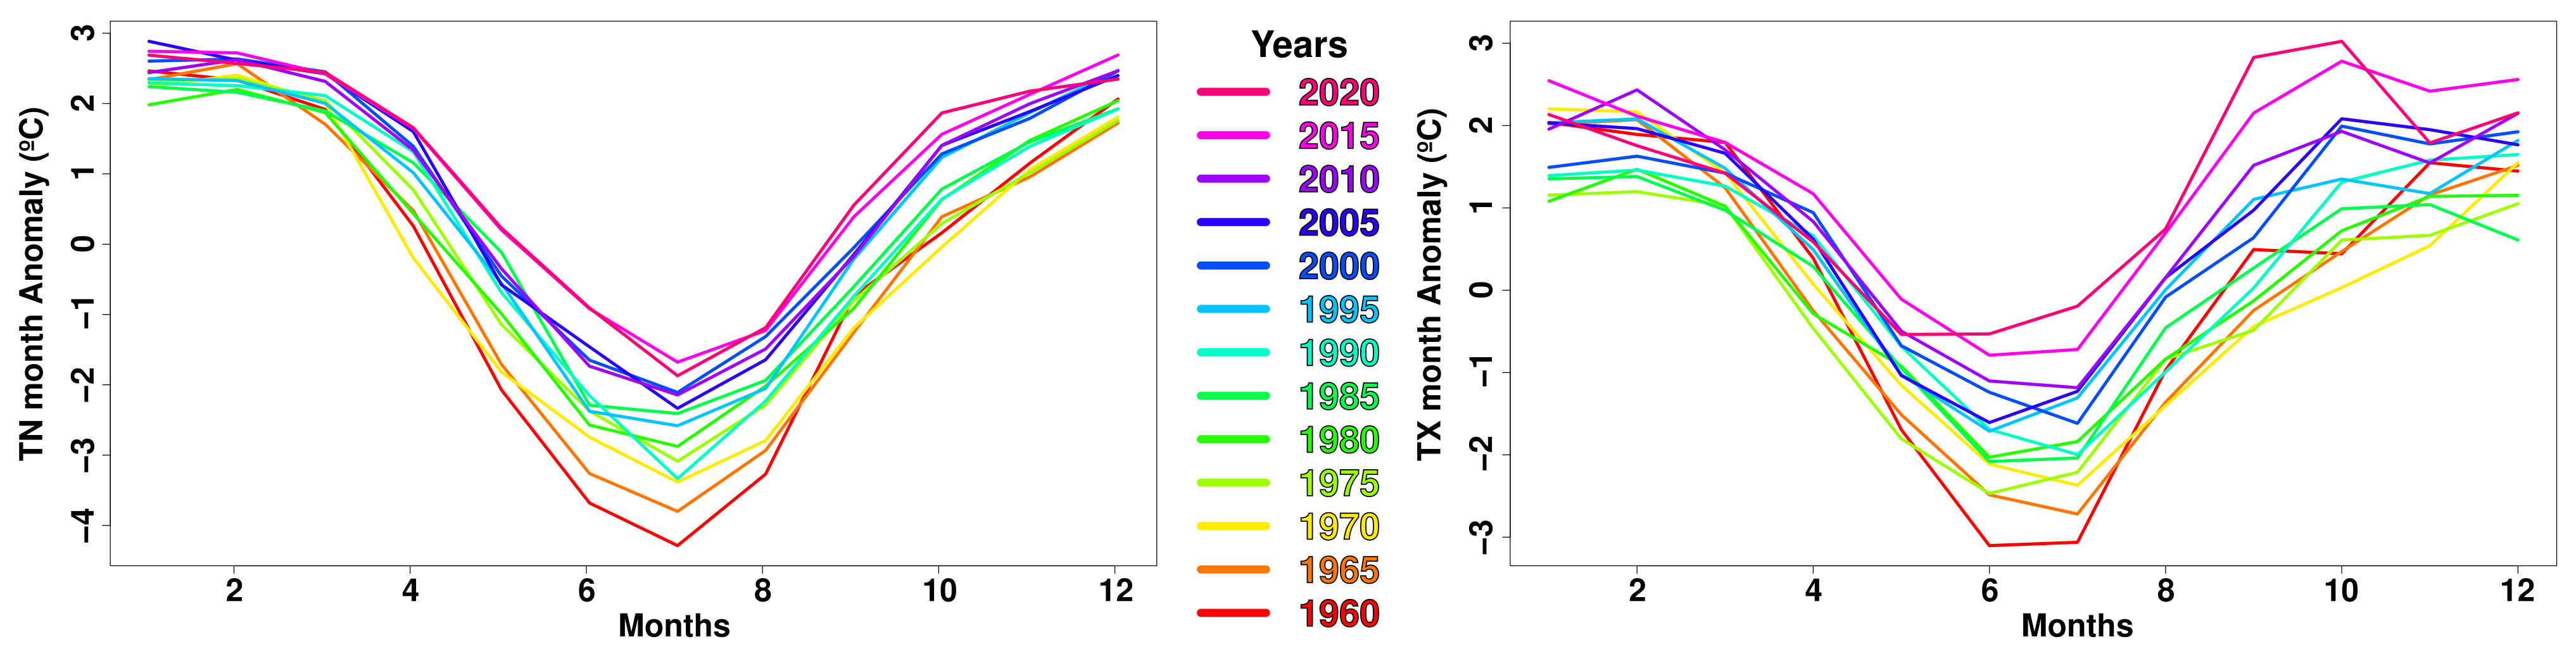}
    \caption{Month anomaly 5 year average in Brazil: left) Minimum temperature anomaly and right) Maximum temperature anomaly. Color code: 5 year average from 1960 (red line) to 2020 (purple line). }
    \label{fig_month_anomaly}
\end{figure}

\begin{figure}[h!]
    \centering
    \includegraphics[width = \textwidth]{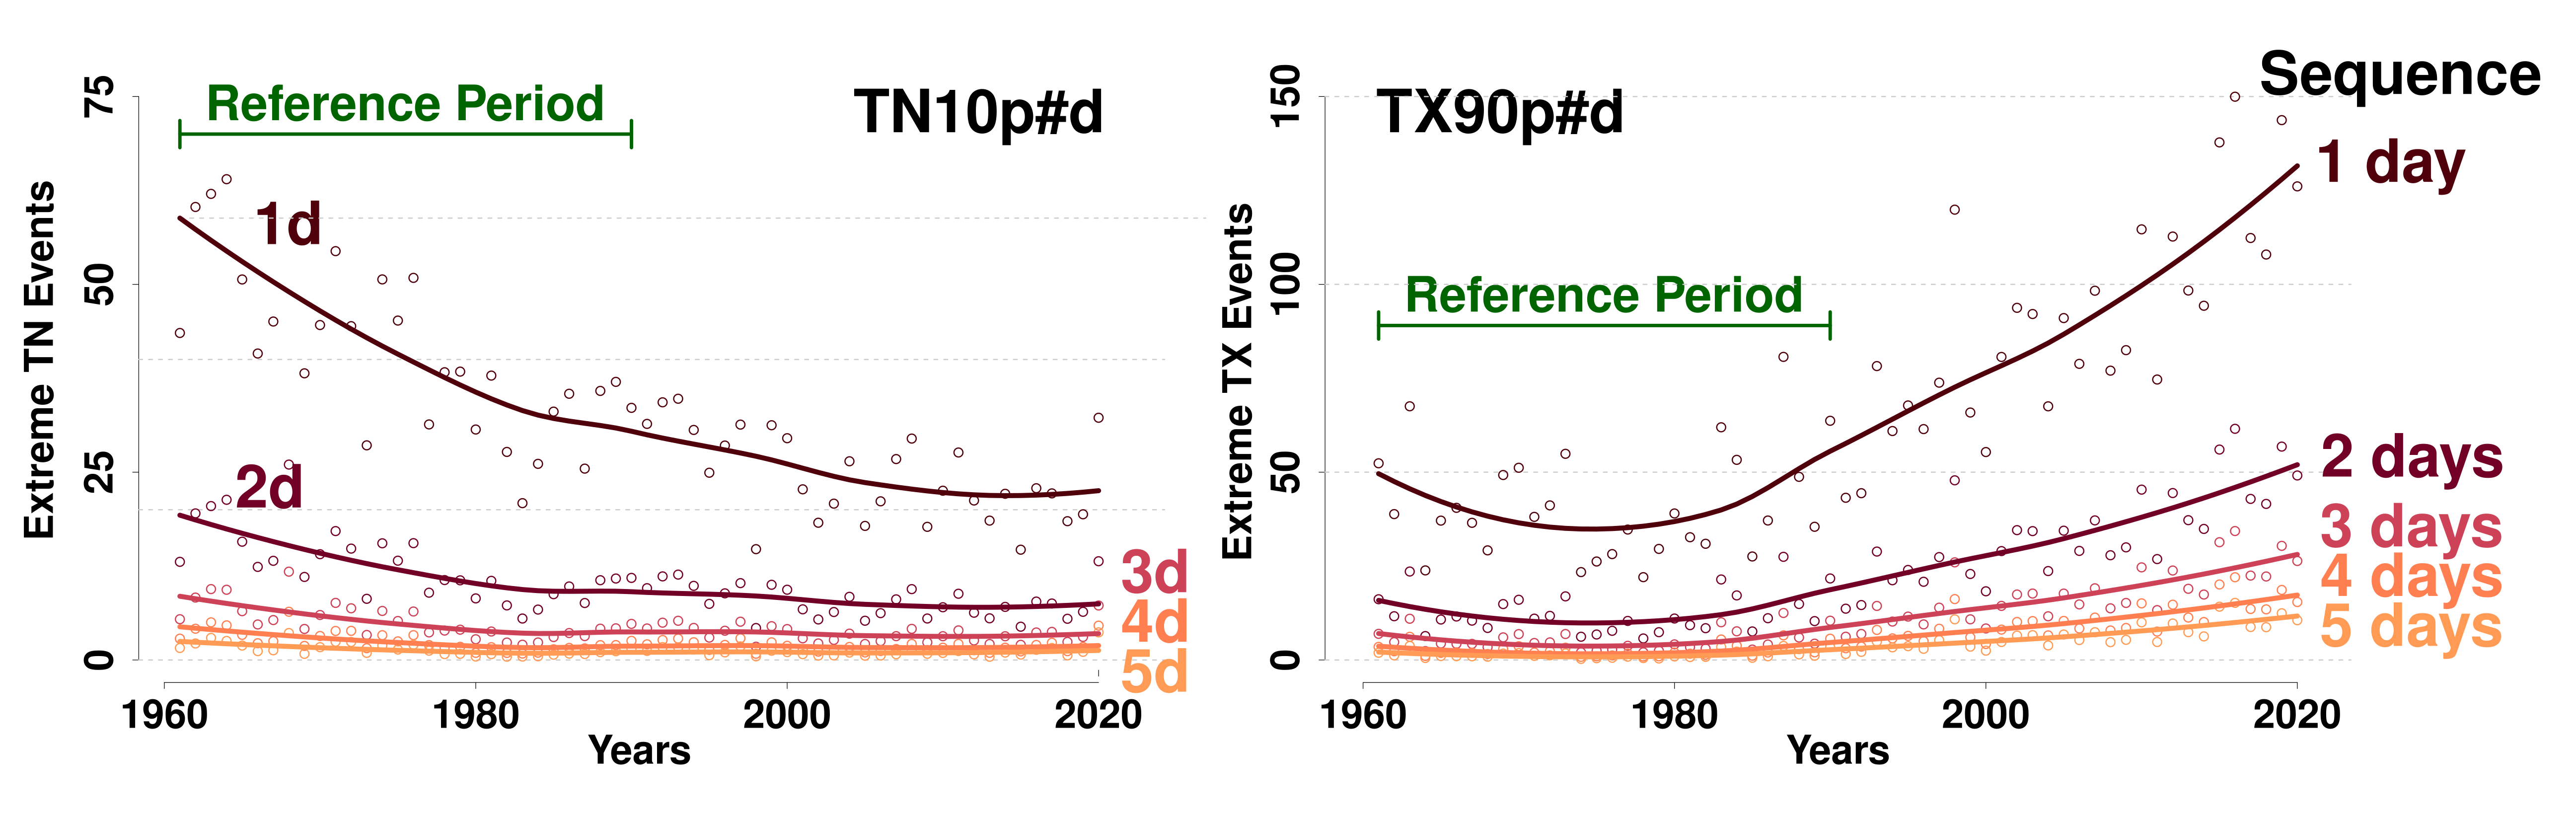}
    \caption{Extreme temperature events by station, for minimum temperature on the left, and maximum temperature on the right. Color-coded for the continuity of events occurrence in days, from wine (1 day) to orange (5 days).}
    \label{fig_temp_extremes}
\end{figure}

To test the robustness of our findings, we have investigated indices more closely related to cold/heat waves, that take into account the temporal continuity of an extreme event. In Figure \ref{fig_temp_extremes} we present the average of EE that have happened $n$ consecutive days: on the Fig. \ref{fig_temp_extremes}-left for the minimum temperature EE, TN10p$n$d, and on the Fig. \ref{fig_temp_extremes}-right for the maximum temperature EE, TX90p$n$d, for $n$ = 1, 3 and 5. We see that the differences in EE consecutiveness do not change much the overall shape of the curves, but decrease their occurrences, as we should expect from more rare (or longer) events. 

\subsection*{Precipitation} \label{precipitation}

Figure \ref{fig_trends_brazil_map} shows the geolocalized precipitation trends for 6 indices. It is possible to see that for a bigger time window (12 months, SPI12 and SPEI12) the points are sparser, since gaps on the data make it unviable to compute the trends. Nevertheless, those trends confirm the overall trend shown in Fig. 3 on the main text.

\begin{figure}[h!]
    \centering
    \includegraphics[width = \textwidth]{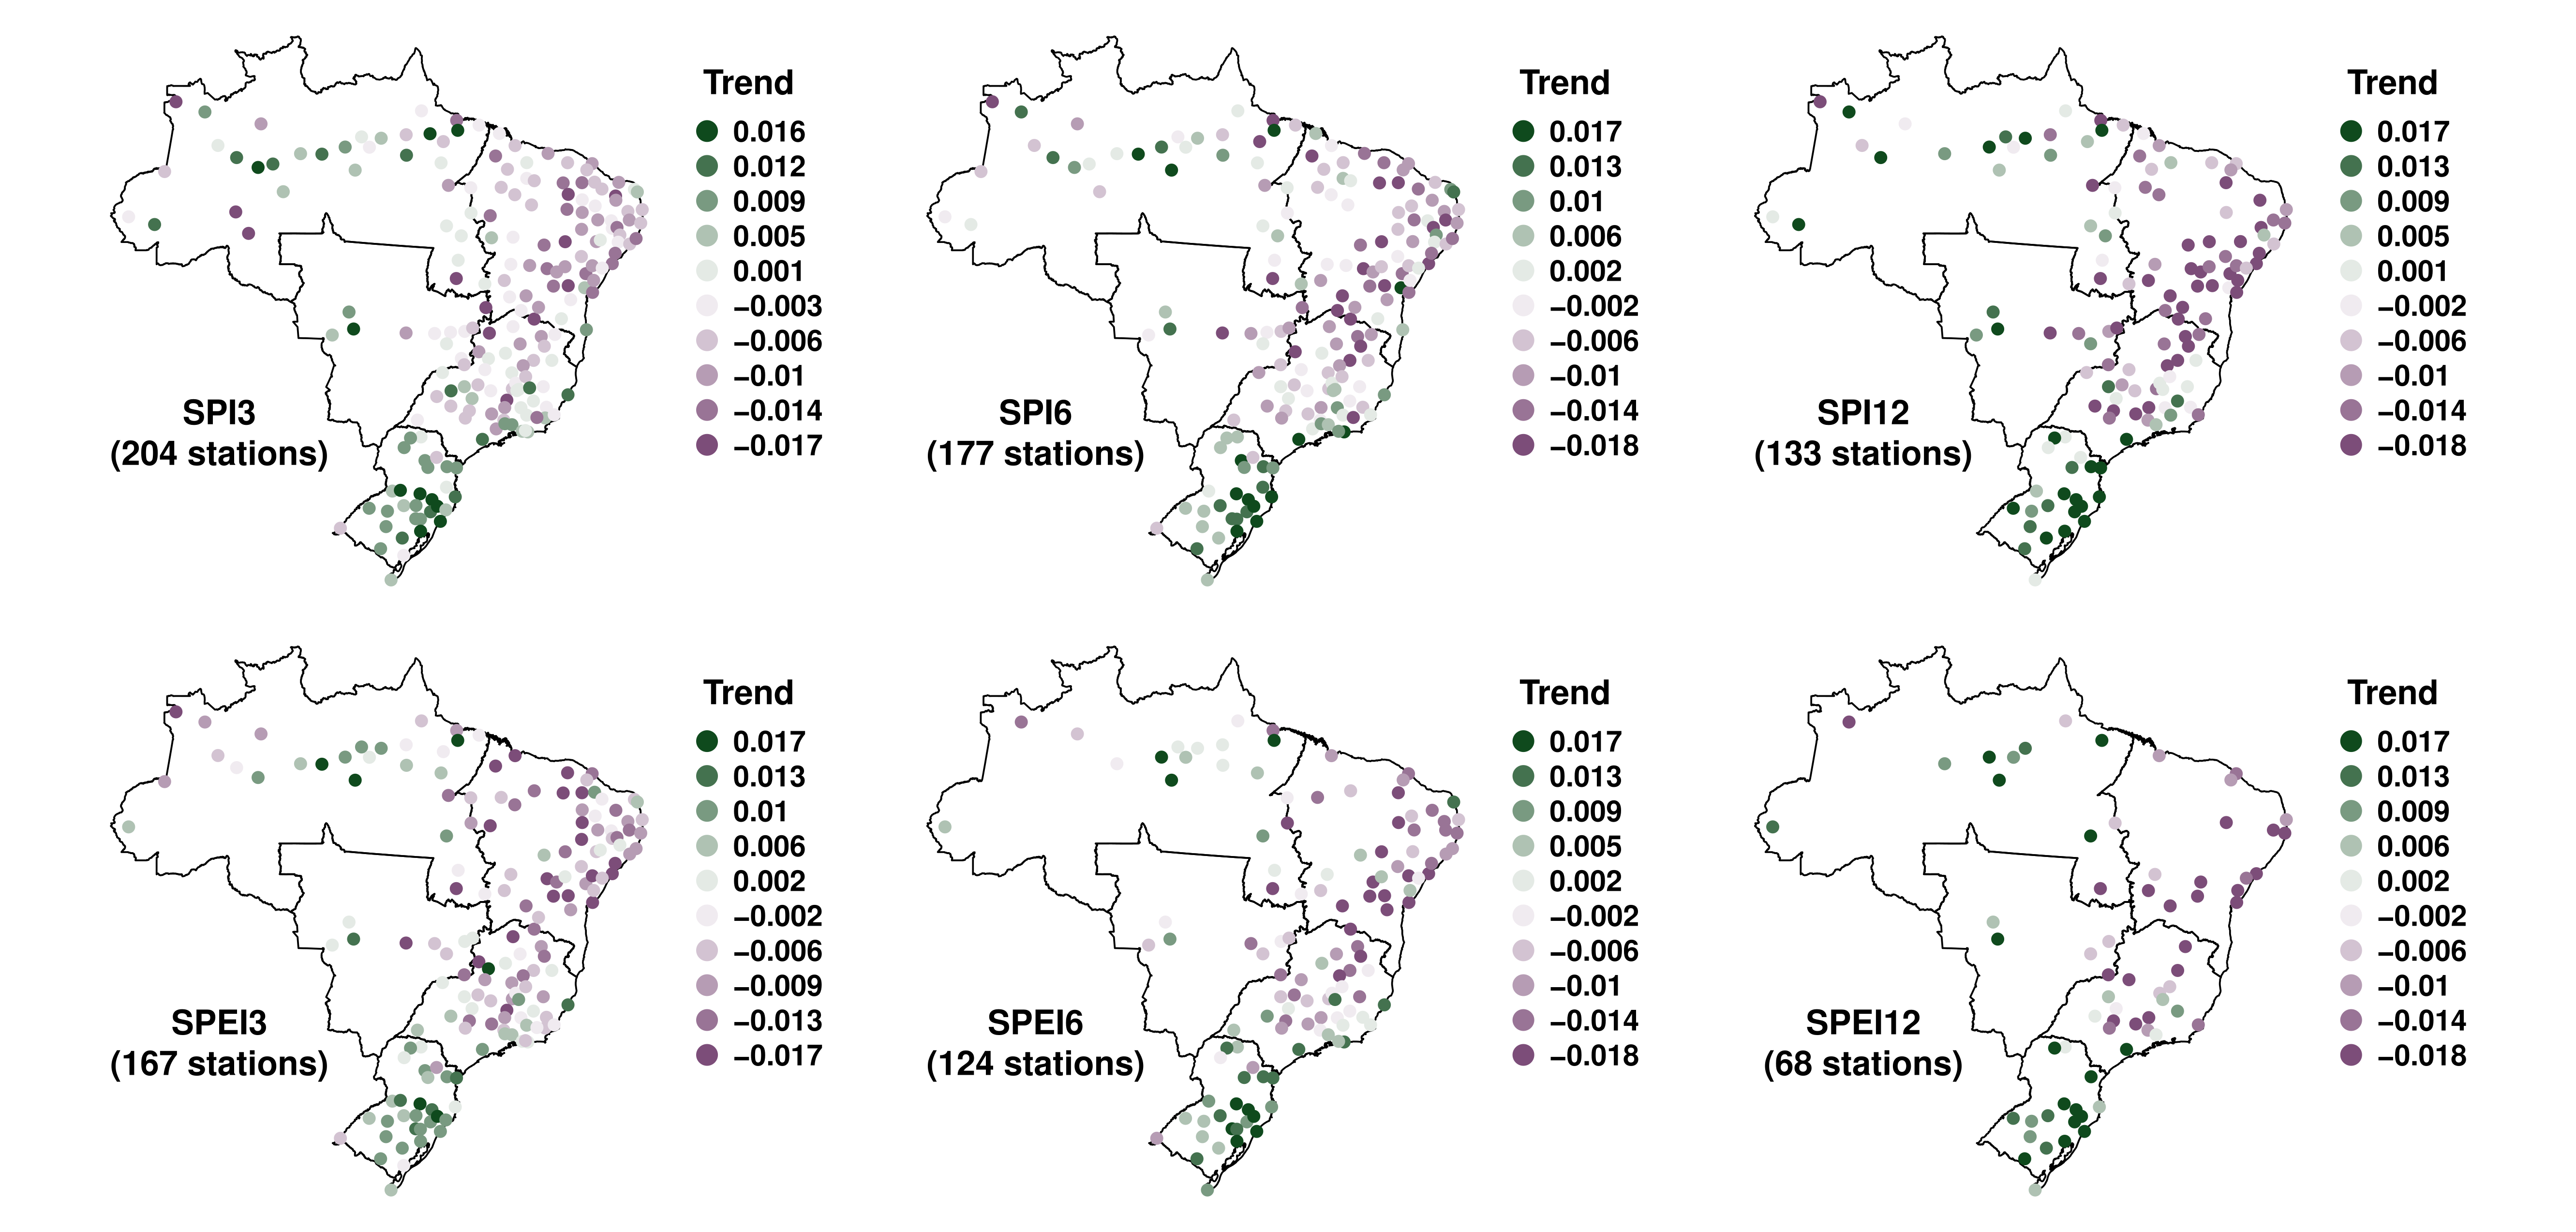}
    \caption{Trends on Standard Precipitation [Evapotranspiration] Indices (SP[E]I): Tendencies of drier/wetter precipitation series geolocalized in Brazil. The number behind the index indicates the time window considered to calculate the precipitation self-correlation series. The points indicate in green the meteorological stations that are becoming wetter, while purple points indicates the stations that are becoming drier.}
    \label{fig_trends_brazil_map}
\end{figure}

\begin{figure}[h!]
    \centering
    \includegraphics[width = .5\textwidth]{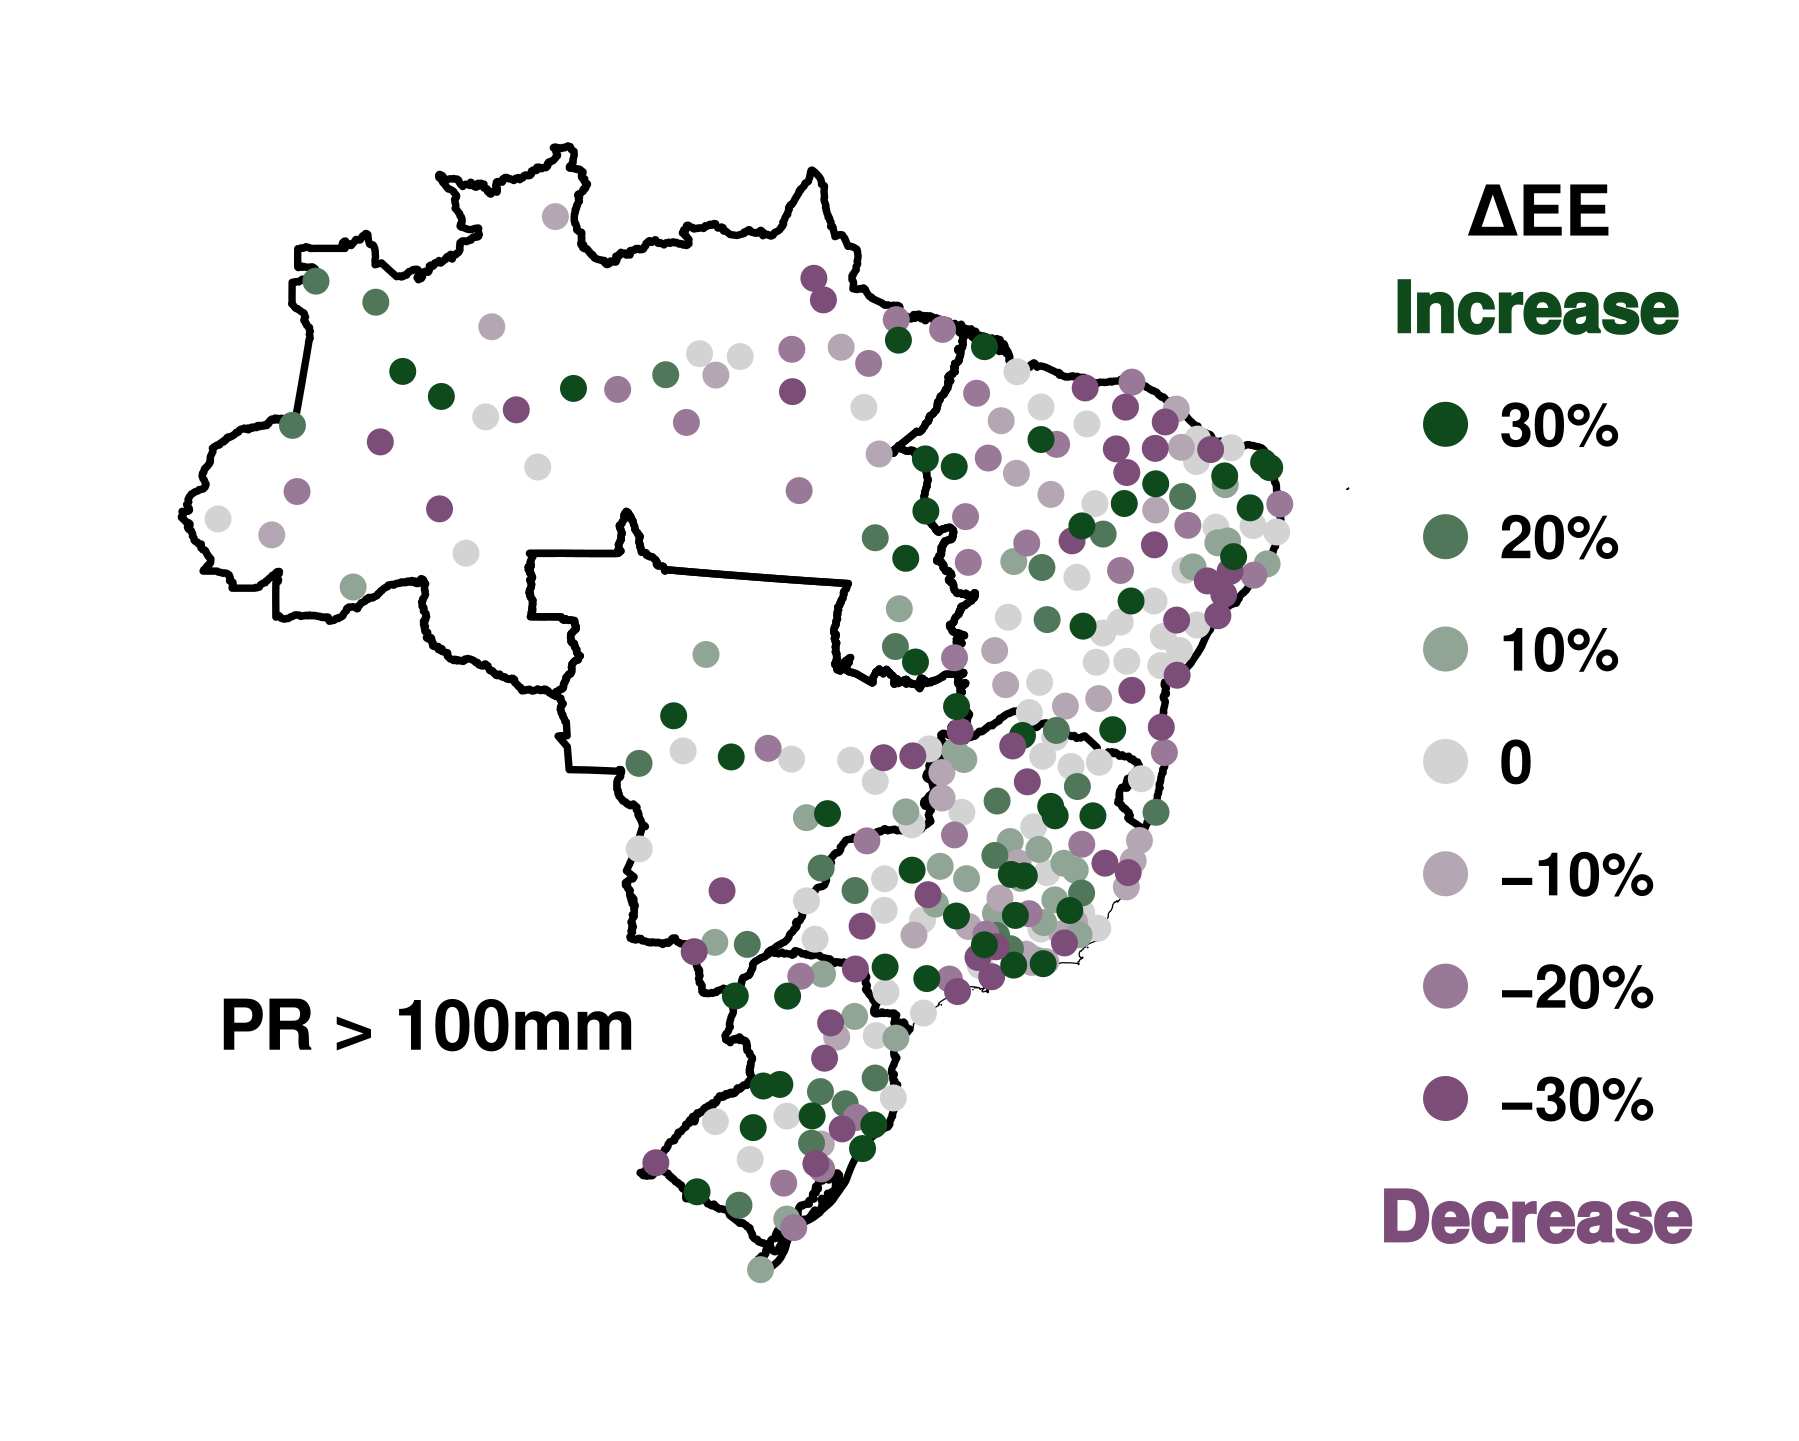}
    \caption{Geolocalized trends of increasing (in green, resp. decreasing in purple) extreme events of precipitation above 100m for each meteorological station.}
    \label{fig_rain_100mm}
\end{figure}

The Figure \ref{fig_rain_100mm} shows the same geolocalized representation for an absolute index, which analyses the extreme precipitation events that present PR $>$ 100mm. The behavior seen is the same as the extreme precipitation map shown on the main text, but with a little more noise, since some meteorological stations do not have enough data (or precipitation) to present signal on this index. This, along with the SPI and SPEI indices, show the robustness of the data presented in the main text, where we show that the north and south regions seem to be getting wetter while the other regions seem to get drier, particularly northeast region, for all the indices.

Figures \ref{fig_drought_regions} and \ref{fig_rain_regions} represent EE time series, measured as defined in Eq. \ref{eq_serietemporal}, separated by different political regions in Brazil. The red lines represent each region's overall trend in events. As they are an average over multiple stations in each region, the behaviors shown are not as clear. 
Due to the average taken over a large region, trend behaviors may be swept away by the average.

\begin{figure}[h!]
    \centering
    \includegraphics[width = 1\textwidth]{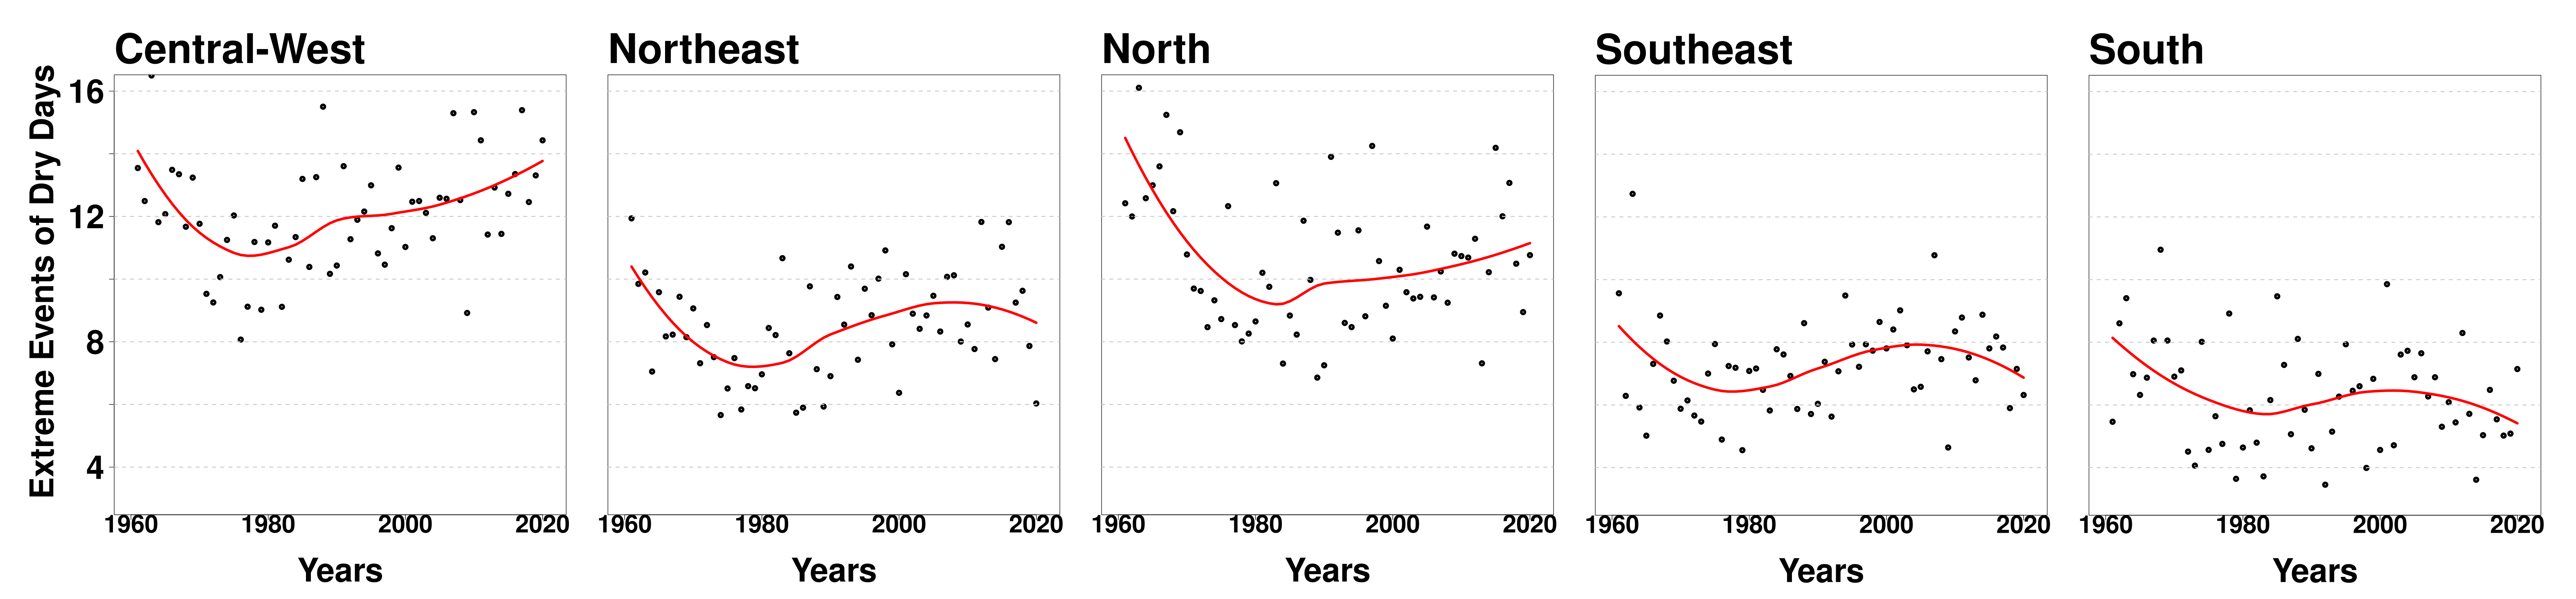}
    \caption{Dry Days extreme events shown as time series separated by Brazilian political regions. The black dots indicate the yearly mean EE and the red lines indicate their trend.}
    \label{fig_drought_regions}
\end{figure}

\begin{figure}[h!]
    \centering
    \includegraphics[width = 1\textwidth]{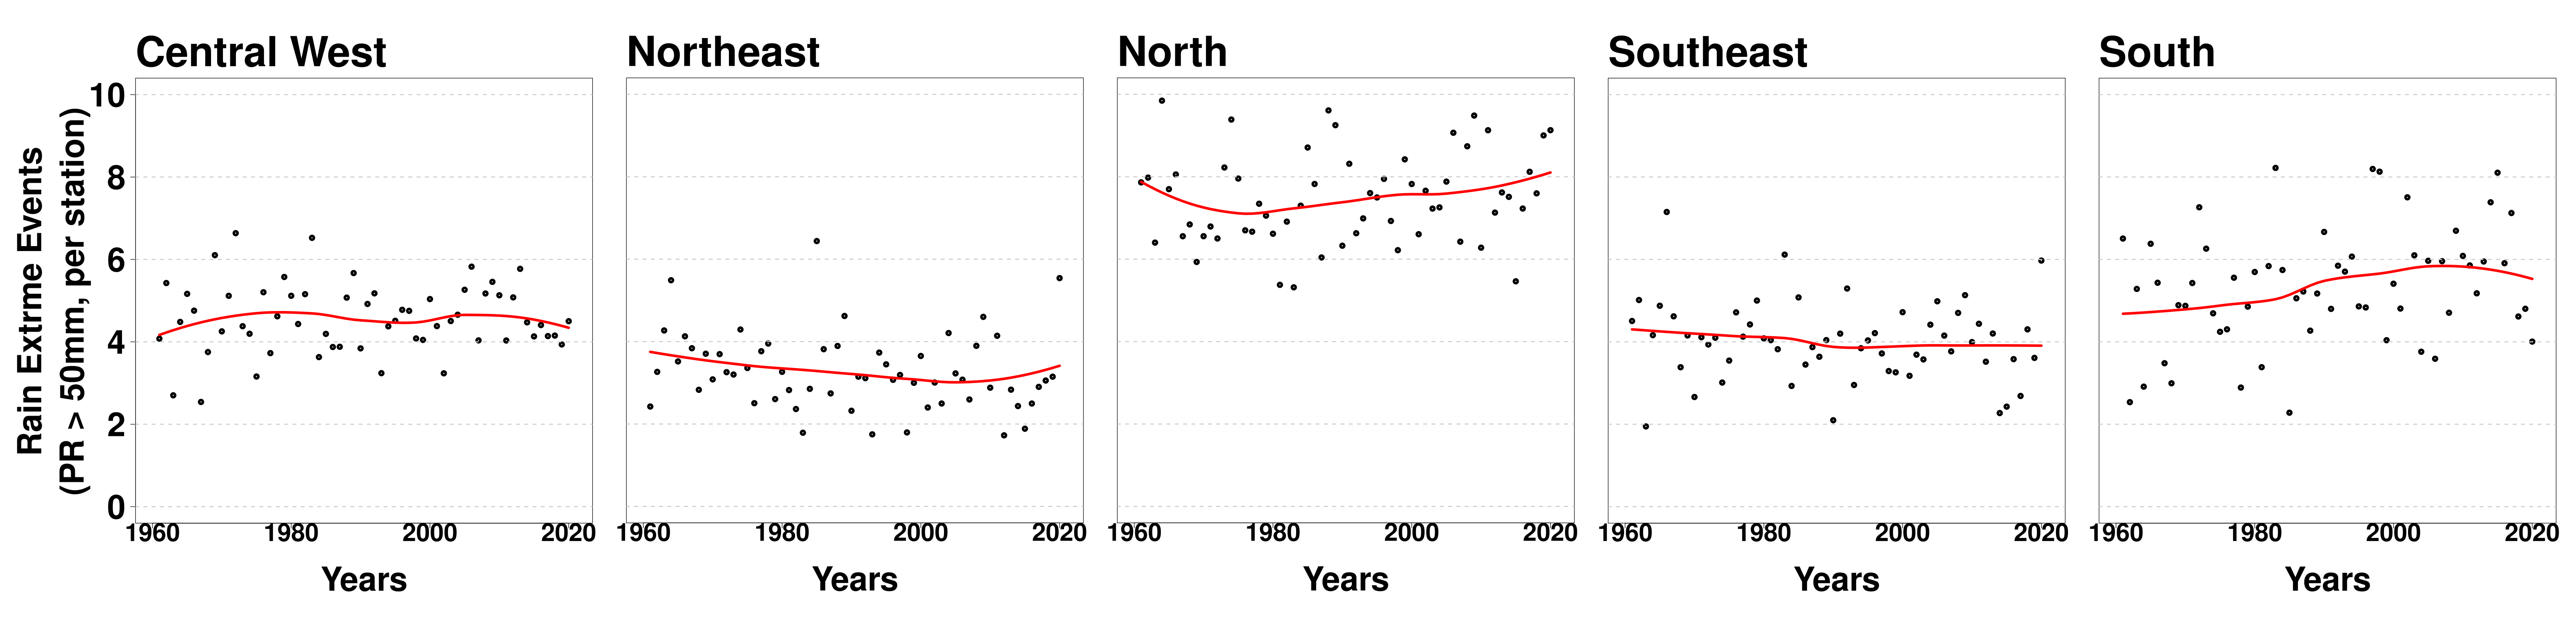}
    \caption{Rain extreme events shown as time series separated by Brazilian political regions. The black dots indicate the yearly mean EE and the red lines indicate their trend.}
    \label{fig_rain_regions}
\end{figure}

\clearpage

\printbibliography

\end{document}
